# Supplementary material for: Deep perceptual hashing algorithms with hidden dual purpose: when client-side scanning does facial recognition
Source: arXiv:2306.11924 source file (2023-06-20)
Supplement: Supplementary file 1 [file notations.tex]

\section{}

This is the set of all notations used in the paper.

\begin{center}[!h]
\begin{tabular}{|c|l|}
    \hline
    Symbol & Description\\
    \hline
    $H$ & Perceptual hashing algorithm\\
    $D$ & Database\\
    $T$ & Threshold\\
    $X$ & Input image\\
    $E$ & Output hash/embedding\\
    $\mathcal{I}$ & Set of all images\\
    $l$ & Length of hash vector\\
    $O$ & Range of an element in hash vector\\
    $f$ & Distance function\\
    $Q$ & Set of query images\\
    $q_i$ & Query image $i$\\
    $R$ & Set of reference images\\
    $r_i$ & Reference image $i$\\
    $I_T$ & Person of interest\\
    $N$ & Number of images available for $I_T$\\
    $H_d$ & Dual-purpose perceptual hashing\\
        & algorithm\\
    $D_d$ & Dual-purpose database\\
    $I$ & Individual $I$\\
    $n_I$ & Number of images for individual $I$\\
    $M_I$ & Images of individual $I$\\
    $F$ & Face detection and recognition\\
    &  algorithm for mislabelled image detection.\\
    $T_{mis}$ & Threshold for mislabelled image\\
    & detection\\
    $S$ & SSCD Algorithm\\
    $T_{dup}$ & Threshold for duplicate detection\\
    $L_{c}$ & Contrastive loss with cross-batch memory\\
    $M$ & Size of cross-batch memory\\
    $A_{m}$ & Moderate augmentations\\
    $A_{h}$ & Hard augmentations\\
    $D_{tr,icd}$ & Training dataset for single-purpose models\\
    
    \hline
\end{tabular}
\end{center}
